# Supplementary material for: Looking for Clues of Language in Multilingual BERT to Improve Cross-lingual Generalization
Source: arXiv:2010.10041 source file (2021-11-01)
Supplement: Supplementary file 1 [file appendix-orig.tex]

\appendix

\section{Analysis of Weight $\alpha$ in Unsupervised Token Translation}


\label{sec:appendix}
\input{sections/tables/common}
\input{sections/tables/en-el.tex}
\begin{figure}[h]
    \centering
    \includegraphics[width=1.0\linewidth]{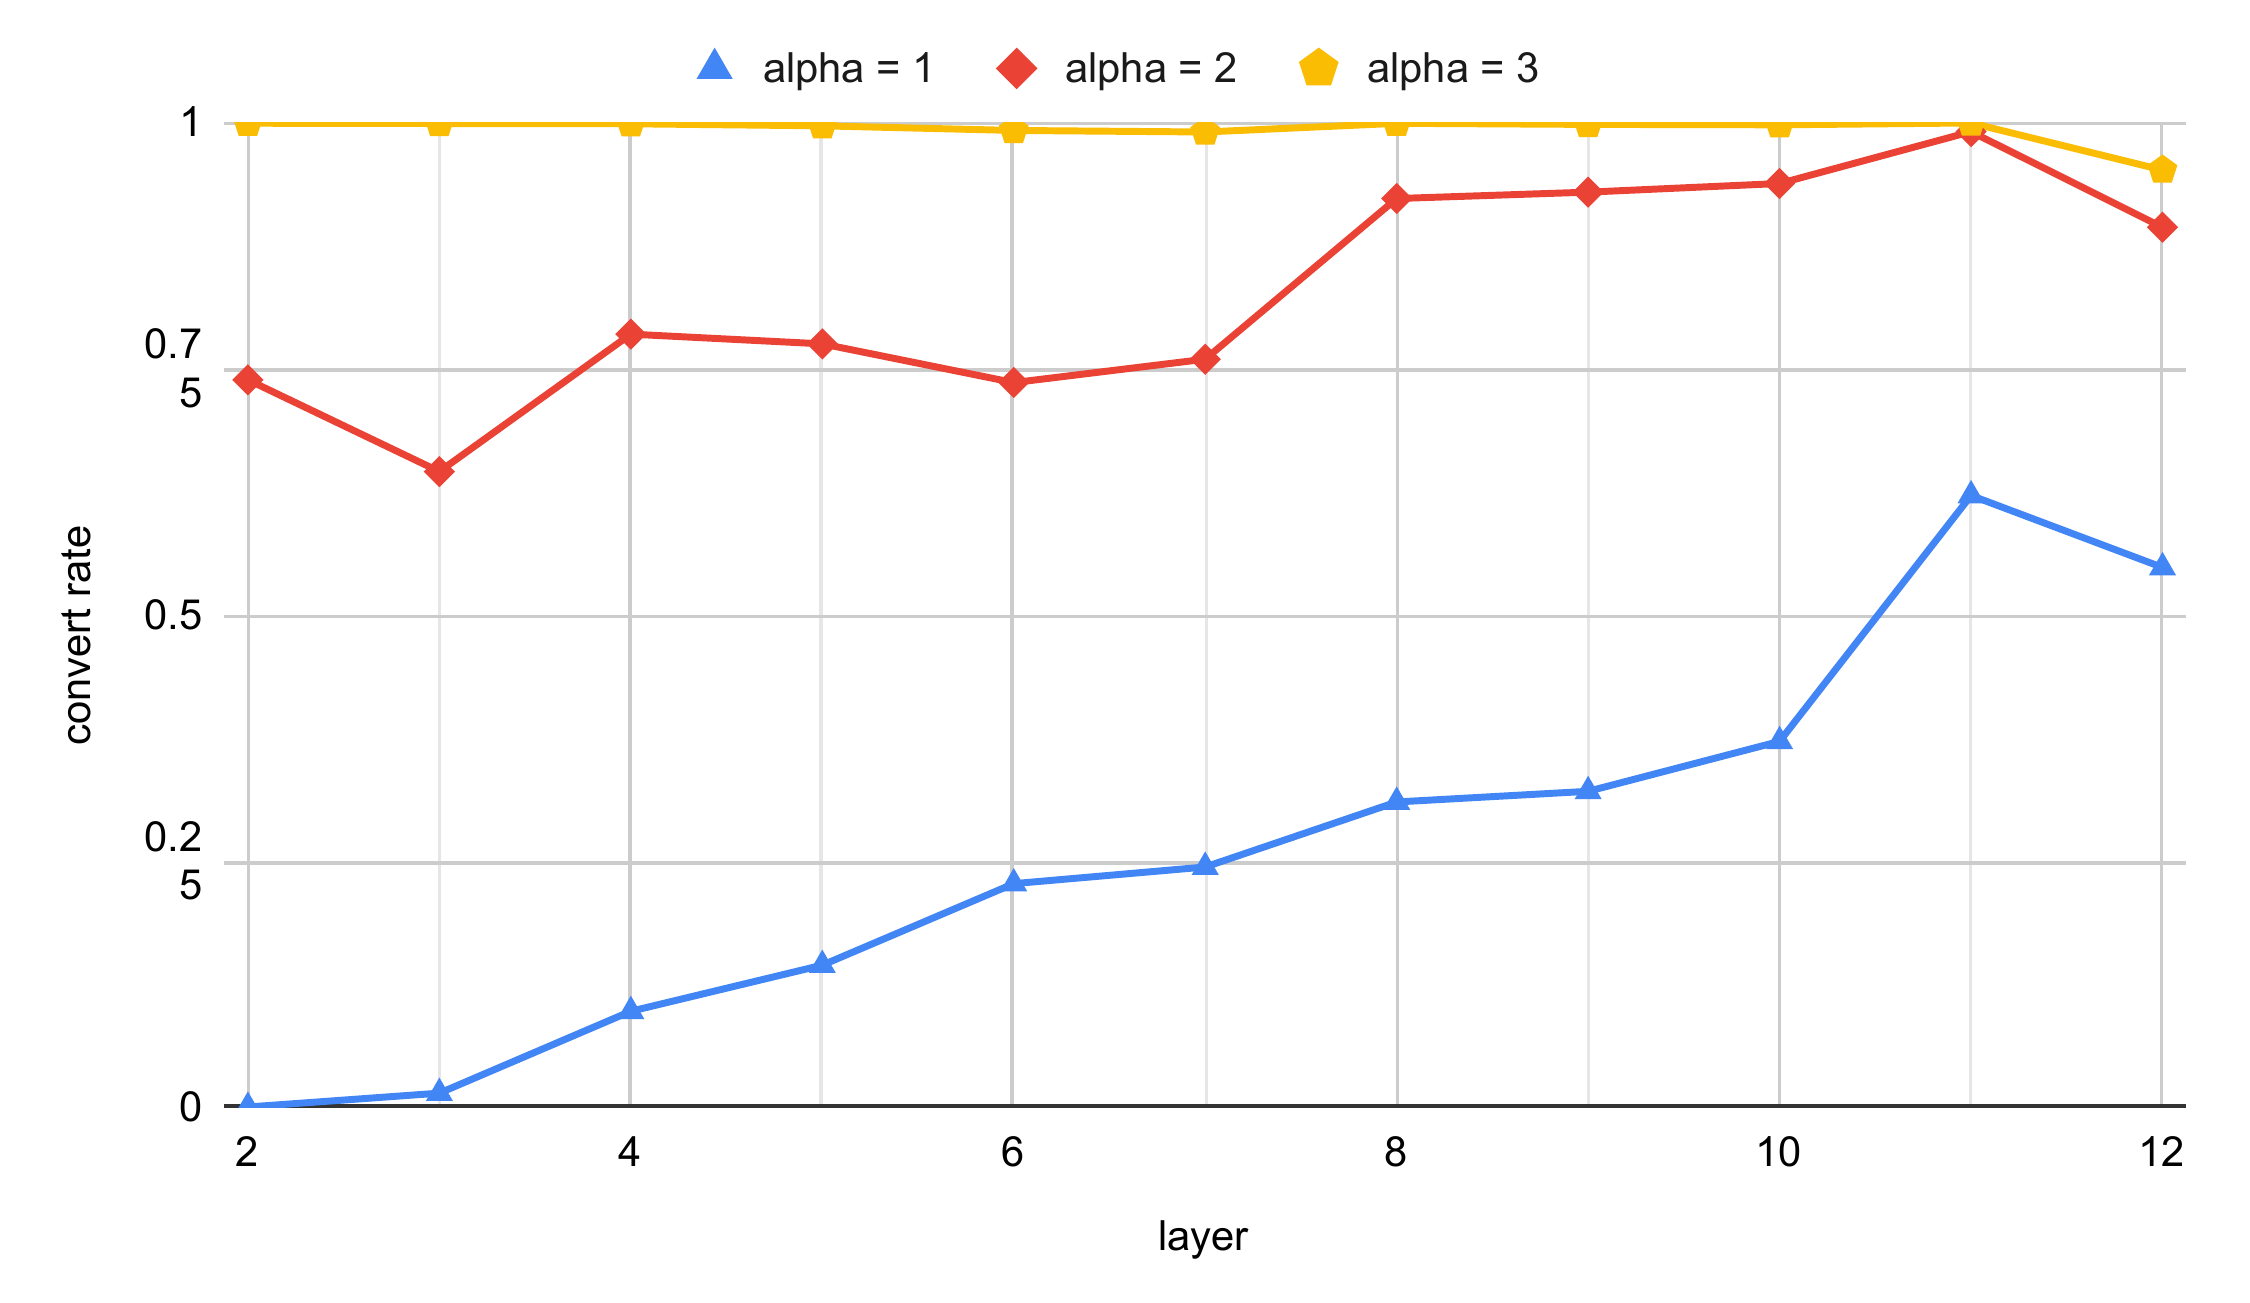}
	 \caption{Convert rate on \textit{en $\veryshortarrow$ el} data when
	 applying different $\alpha$ on different layers for MDS.}
    \label{fig:convert}
\end{figure}
\input{sections/tables/examples}

We present an example of \textit{en $\veryshortarrow$ el} in an
Figure~\ref{fig:convert} and~\ref{fig:bleuchange} show that how convert rate
and BLEU-1 score changed with different weights $\alpha$ and different layers. 


Although, the influences of weight increase on BLEU-1 score were mixed, it is
worth mentioning that in the last few layers (10 or 11), the BLEU-1 of most
languages obviously rose when $\alpha$ was set to $3.0$ (also shown in the best
layer row in Table~\ref{tab:mt}). 
It indicates that the last few layers may be better for disentangling
language-specific representations, which is consistent with the observation in
the literature that the last few layers contain more language-specific
information for predicting masked words~\citep{pires:19}.

% \section{Difference between MDS and Zero Mean}
% \label{sec:mds_zm_diff}
% Assume we have sentence representation $\vect{v_1}\in$ Language $L_1$ and $\vect{v_2}\in L_2$, and the approximate language representation  $\hat{\vect{R}_{L_1}}$ and~$\hat{\vect{R}_{L_2}}$ and real language representation $\vect{R}_{L_1}$ and~$\vect{R}_{L_2}$. $\delta_1$ and $\delta_2$ are difference between approximate language representation and real language representation. We suppose that $\vect{v}_1$ and $\vect{v}_2$ are the same after applying MDS or Zero-Mean.
% \[
% \begin{split}
%     &\vect{v}_1-\vect{R}_{L_1}=\vect{v}_2-\vect{R}_{L_2} \\
%   \rightarrow& \vect{v}_1-\hat{\vect{R}}_{L_1}-\vect{\delta}_1=\vect{v}_2-\hat{\vect{R}}_{L_2}-\vect{\delta}_2
% \end{split}
% \]
% As a result, we have

% \[
% \small
% \begin{split}
% \cos_\text{MDS}\left(\vect{v_1},\vect{v_2}\right)
% &= \frac{ \left(\vect{v}_1-\hat{\vect{R_{L_1}}}+\hat{\vect{R_{L_2}}}\right) \cdot \vect{v_2}}
% {\left\lvert\vect{v}_1-\hat{\vect{R_{L_1}}}+\hat{\vect{R_{L_2}}}\right\rvert\left\lvert\vect{v}_2\right\rvert}\\
% &= \frac{ \left(\vect{v}_2+\vect{\delta}\right) \cdot \vect{v_2}}
% {\left\lvert \vect{v}_2+\vect{\delta}\right\rvert\left\lvert\vect{v}_2\right\rvert}, \text{ where } \vect{\delta}=\vect{\delta}_1-\vect{\delta}_2\\\
% \cos_\text{ZeroMean}\left(\vect{v_1},\vect{v_2}\right)
% &= \frac{ \left(\vect{v}_1-\hat{\vect{R_{L_1}}}\right) \cdot \left(\vect{v_2 -\hat{\vect{R_{L_2}}} }\right)}
% {\left\lvert\vect{v}_1-\hat{\vect{R_{L_1}}}\right\rvert\left\lvert\vect{v}_2-\hat{\vect{R_{L_2}}}\right\rvert}\\
% &= \frac{
% \left(\vect{v_2}- \vect{R_{L_2}} + \vect{\delta}_1\right) \left(\vect{v_2}- \vect{R_{L_2}} + \vect{\delta}_2\right)}
% {\left\lvert\vect{v_2}- \vect{R_{L_2}} + \vect{\delta}_1\right\rvert \left\lvert\vect{v_2}- \vect{R_{L_2}} + \vect{\delta}_2\right\rvert}\\
% \end{split}
% \]

% The above result shows that Zero-Mean method is more sensitive to the approximate error when $\left\lvert\vect{v_2} \right\rvert > \left\lvert\vect{v_2}- \vect{R_{L_2}}\right\rvert > \max\left(\abs{\vect{\delta_1}}, \abs{\vect{\delta_2}}, \abs{\vect{\delta}}\right)\geq 0$.
%$\vect{m_1},\vect{m_2}$ are the mean vector of representations in $L_1$ and $L_2$ separately. Then the cosine similarity between shifted $\vect{v_1}\in$ and $\vect{v_2}\in$ can be written as: 

% \paragraph{Contextualized Word Retrieval}
% The contextualized word retrieval task was formulated as such: given a token representation~$\vect{h}^l_{x_i}$, retrieve its k-nearest neighbors in the representation space $KNN = \vect{h}^l_{y_j}, \vect{h}^l_{z_k} ...$, with cosine similarity. 
% Given a bilingual dictionary~$D=\{(t_1,t_2),(t_3,t_4),\ldots\}$, where $t_1, t_2, ...$ are token types in the vocabulary of m-BERT, and then the evaluation metric mean-reciprocal rank~(MRR) on the retrieval result of token $x_i$ was calculated as such: 
% \begin{equation}
% \text{MRR$_{x_i}$} = \sum\frac{1}{\text{rank$_{KNN}$}(y_j)}, 
% \end{equation}
% where the summation was over all token $y_j$ whose token type $t_{y_j}$ is a translation of $t_{x_i}$, that is, $(t_{x_i},t_{y_j})$ is in $D$, and 
% \begin{equation}
% \text{MRR}=average~\text{MRR$_{x_i}$}
% \end{equation}

% We used the bilingual dictionaries from MUSE\footnote{https://github.com/facebookresearch/MUSE} and token representations sampled from XNLI to conduct the contextualized word retrieval experiment. When applying MDS or Zero-mean, shifts were directly added to the layer of token representations used for retrieval. We experimented with MDS and Zero-mean to see if these methods help align words better so that better word retrieval results are achieved. Here we also experimented with linear mapping method from MUSE to draw a comparison. 


% \section{Supplemental Material}
% \label{sec:supplemental}
%\input{sections/tables/word_retrieval}
